# Supplementary material for: Empirical Guidelines for Deploying LLMs onto Resource-constrained Edge Devices
Source: arXiv:2406.03777 source file (2024-10-02)
Supplement: Supplementary file 1 [file appendix_G.tex]

\begin{figure*}[ht]
  \centering
  % First row of figures
  \begin{subfigure}[b]{0.49\textwidth}
    \includegraphics[width=1\textwidth]{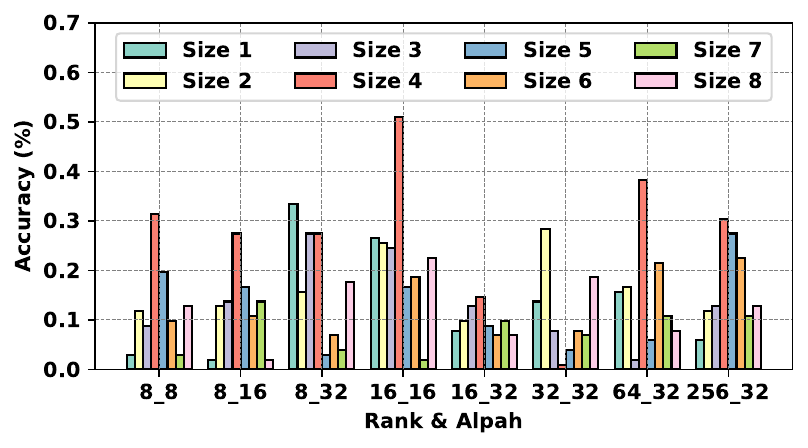}
    \caption{Pythia-410m on LaMP-1}
    \label{fig:a}
  \end{subfigure}
  % \hfill % space between the subfigures
  \begin{subfigure}[b]{0.49\textwidth}
    \includegraphics[width=1\textwidth]{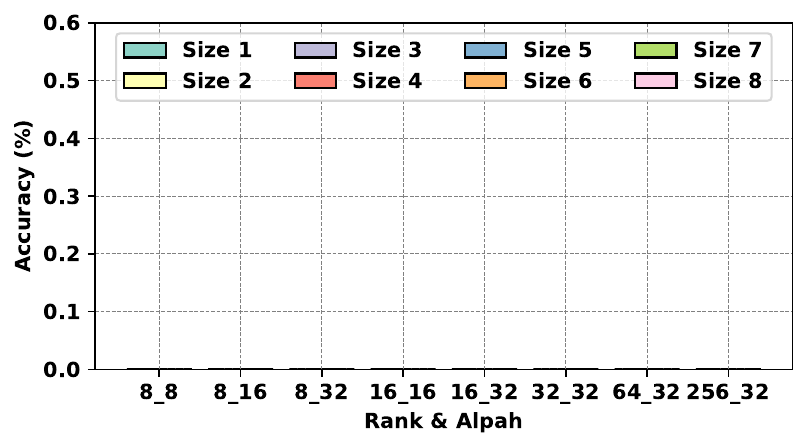}
    \caption{Pythia-410m on LaMP-2}
    \label{fig:b}
  \end{subfigure}
  % \hfill % space between the subfigures
  \begin{subfigure}[b]{0.49\textwidth}
    \includegraphics[width=1\textwidth]{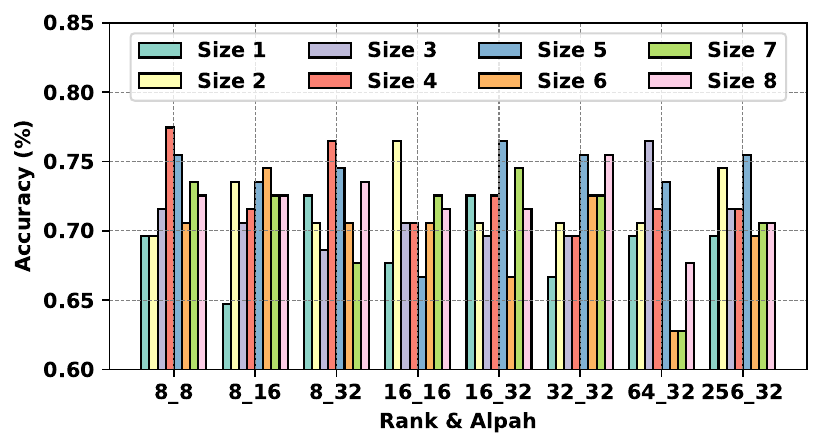}
    \caption{Pythia-410m on LaMP-3}
    \label{fig:c}
  \end{subfigure}
  % Second row of figures
  \begin{subfigure}[b]{0.49\textwidth}
    \includegraphics[width=1\textwidth]{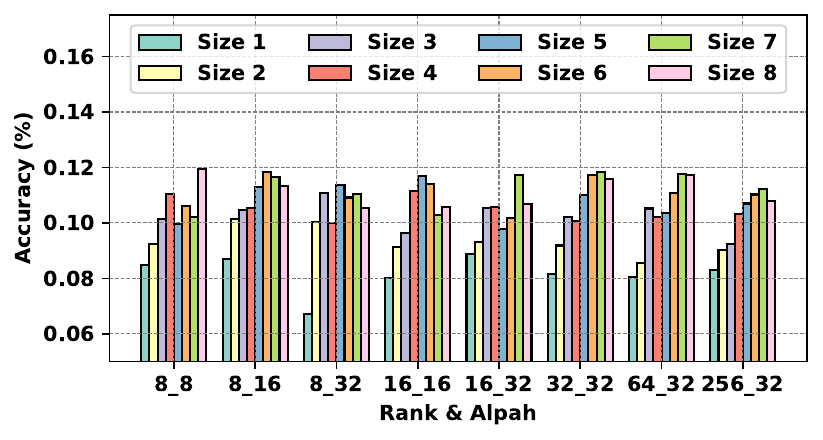}
    \caption{Pythia-410m on LaMP-4}
    \label{fig:d}
  \end{subfigure}
  % \hfill % space between the subfigures
  \begin{subfigure}[b]{0.49\textwidth}
    \includegraphics[width=1\textwidth]{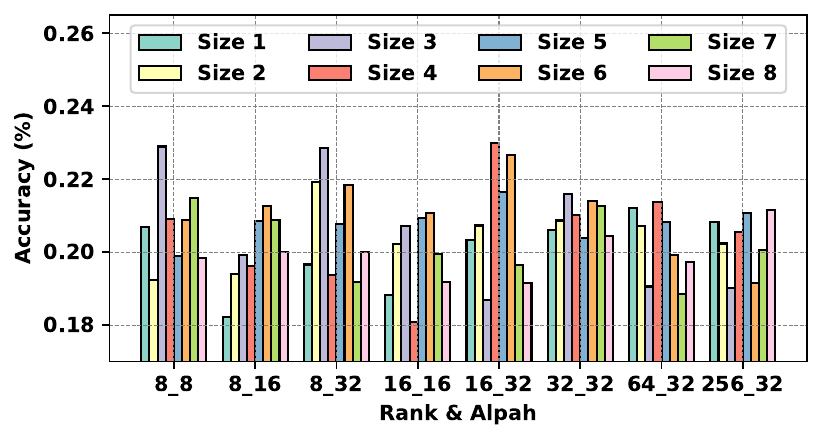}
    \caption{Pythia-410m on LaMP-5}
    \label{fig:e}
  \end{subfigure}
  % \hfill % space between the subfigures
  \begin{subfigure}[b]{0.49\textwidth}
    \includegraphics[width=1\textwidth]{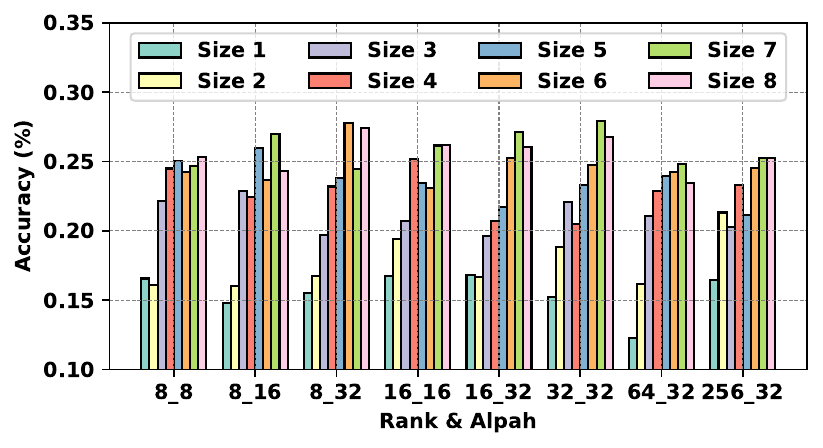}
    \caption{Pythia-410m on LaMP-6}
    \label{fig:f}
  \end{subfigure}
    % \hfill % space between the subfigures
  \begin{subfigure}[b]{0.49\textwidth}
    \includegraphics[width=1\textwidth]{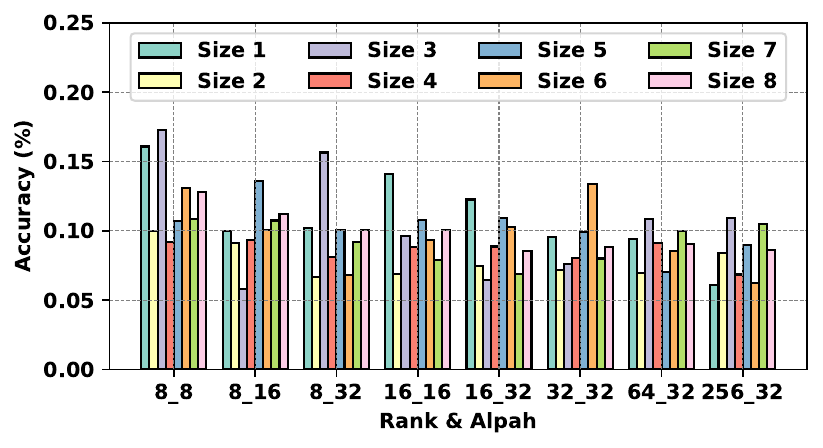}
    \caption{Pythia-410m on LaMP-7}
    \label{fig:g}
  \end{subfigure}

  \caption{\rqin{Caption is need}}
  \label{fig:b-1-1-1}
\end{figure*}

\begin{figure*}[ht]
  \centering
  % First row of figures
  \begin{subfigure}[b]{0.49\textwidth}
    \includegraphics[width=1\textwidth]{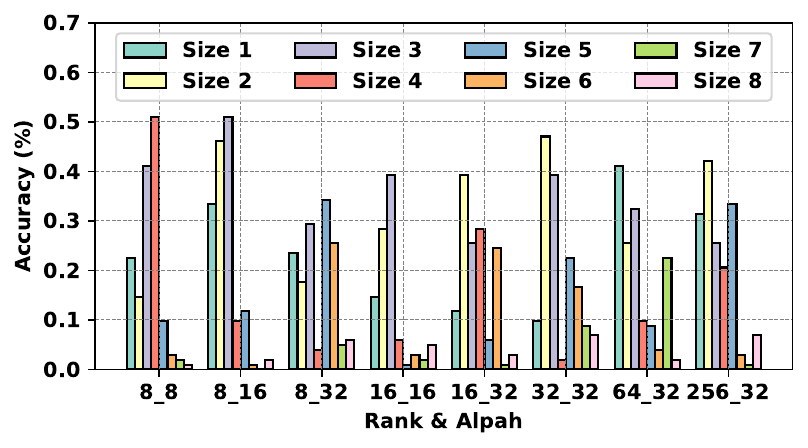}
    \caption{Pythia-1b on LaMP-1}
    \label{fig:a}
  \end{subfigure}
  % \hfill % space between the subfigures
  \begin{subfigure}[b]{0.49\textwidth}
    \includegraphics[width=1\textwidth]{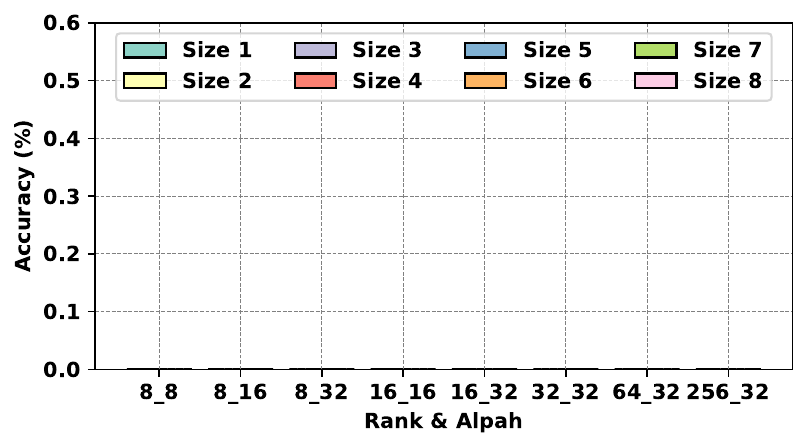}
    \caption{Pythia-1b on LaMP-2}
    \label{fig:b}
  \end{subfigure}
  % \hfill % space between the subfigures
  \begin{subfigure}[b]{0.49\textwidth}
    \includegraphics[width=1\textwidth]{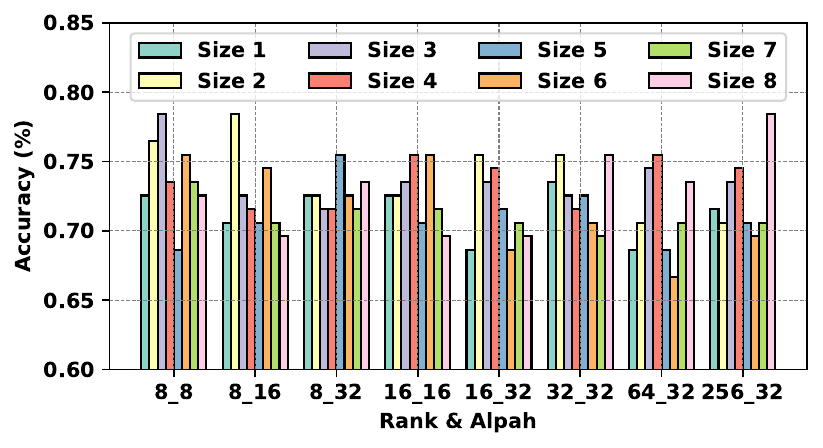}
    \caption{Pythia-1b on LaMP-3}
    \label{fig:c}
  \end{subfigure}
  % Second row of figures
  \begin{subfigure}[b]{0.49\textwidth}
    \includegraphics[width=1\textwidth]{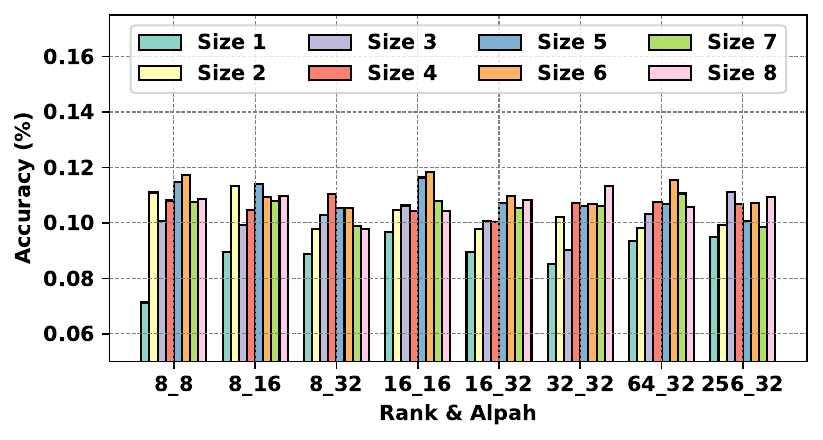}
    \caption{Pythia-1b on LaMP-4}
    \label{fig:d}
  \end{subfigure}
  % \hfill % space between the subfigures
  \begin{subfigure}[b]{0.49\textwidth}
    \includegraphics[width=1\textwidth]{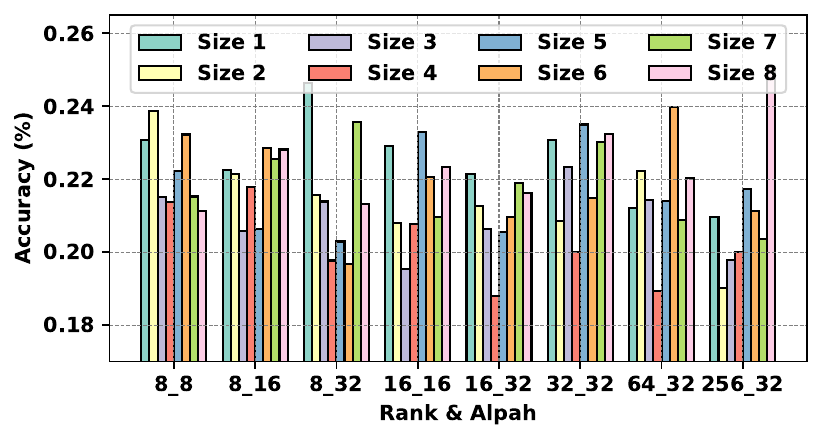}
    \caption{Pythia-1b on LaMP-5}
    \label{fig:e}
  \end{subfigure}
  % \hfill % space between the subfigures
  \begin{subfigure}[b]{0.49\textwidth}
    \includegraphics[width=1\textwidth]{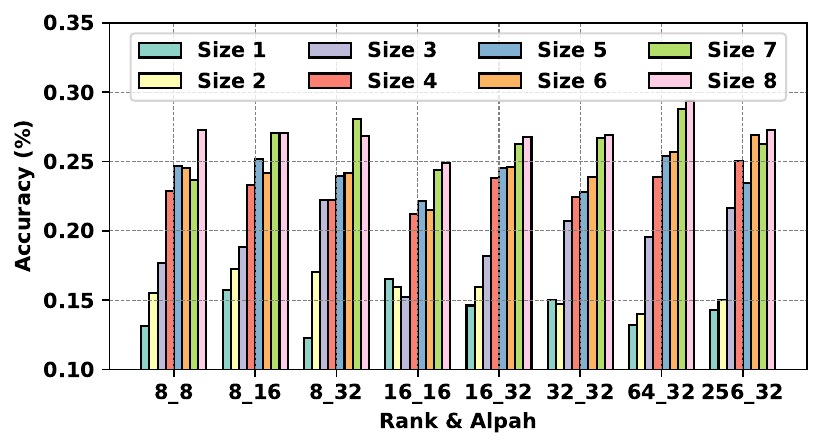}
    \caption{Pythia-1b on LaMP-6}
    \label{fig:f}
  \end{subfigure}
    % \hfill % space between the subfigures
  \begin{subfigure}[b]{0.49\textwidth}
    \includegraphics[width=1\textwidth]{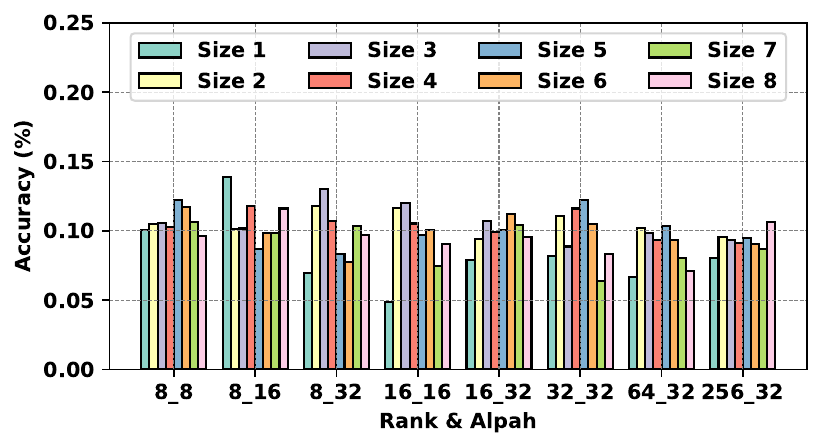}
    \caption{Pythia-1b on LaMP-7}
    \label{fig:g}
  \end{subfigure}

  \caption{\rqin{Caption is need}}
  \label{fig:b-1-1-1}
\end{figure*}
